# Supplementary material for: Nonlinear nonequilibrium quasiparticle relaxation in Josephson junctions
Source: arXiv:0910.0161 source file (2009-10-01)
Supplement: Supplementary file 1 [file KrasnovText_NE_Suppl_v2.pdf]

# Supplementary information to the manuscript: Nonlinear nonequilibrium quasiparticle relaxation in Josephson junctions

V. M. Krasnov
*Department of Physics, Stockholm University, AlbaNova University Center, SE-10691 Stockholm, Sweden*

In this supplementary I present the complete formulation of the problem of nonlinear nonequilibrium quasi-particle and boson relaxation in Josephson junctions, clarify the numerical procedure and, for comparison, show solutions of the linearized version of kinetic equations.

PACS numbers: 74.40.+k 74.50.+r 42.55.Px 85.60.Jb 78.45.+h

## I. DEFINITIONS AND NOMENCLATURE

$D_{QP}(0)$ the quasiparticle density of states per spin at Fermi level $\sim 10^{22}(states/eVcm^3)$ [1].

$D_B(\Omega)$ the boson density of states per ion (1/eV). I intentionally use the simplest Debye approximation for bosons: $D_B(\Omega) = 3\Omega^2/\Omega_D^3$.

$\Omega_D$ the effective bosonic Debye energy, I assumed $\Omega_D \sim 100meV$, because for HTSC there are phonons up to 100 meV [2]. Furthermore, other relevant bosons, like spin waves and plasmons may have even larger energies.

$\alpha^2 D_B(\Omega) \simeq b\Omega^2$ is the effective electron-boson spectral function (scaled with DoS). In the last expression Debye approximation is used. In this case $b \sim \lambda/\Omega_D^2$, where $\lambda$ is the electron-boson coupling constant [3]. Assuming $\lambda \sim 2$ [2], we obtain $b \sim 2 \times 10^2 (eV)^{-2}$.

$\mathfrak{V} = Ad$ volume of electrodes, where $A$ - is the area, and $d$ is the electrode thickness. For Bi-2212 IJJs I assumed $d \simeq 4\mathring{A}$.

$s = 1.5nm$ - the interlayer spacing in Bi-2212

$\Delta$ the average superconducting energy gap. $\Delta_0(T)$ is the equilibrium value of the gap at the base temperature $T$. The gap depends on temperature and for Bi-2212 IJJs ranges from 30 meV at $T = 0$ to 0 at $T_c$ [4]. For estimations of coefficients at intermediate temperatures I assumed $\Delta = 10meV$.

$N_I$ - density of ions. For Bi-2212 $N_I \simeq 2 \times 10^{22} cm^{-3}$.

$v_S$ sound velocity $\sim 4 \times 10^5 cm/s$ [5] is appropriate for phonons. For electronic excitations (spin-waves, plasmons) the velocity is of the order of the Fermi velocity, $v_F$, which is about two order of magnitude larger [6].

$f(E) = \delta f(E) + F(E)$ and $g(\Omega) = \delta g(\Omega) + G(\Omega)$ are the nonequilibrium occupation numbers for quasiparticles and bosons, respectively. Here $F(E,T) = [\exp(E/k_BT) + 1]^{-1}$ and $G(\Omega,T) = [\exp(\Omega/k_BT) - 1]^{-1}$ are the equilibrium Fermi-Dirac and Bose-Einstein distribution functions at the base temperature $T$, respectively, and $\delta f$ and $\delta g$ are the nonequilibrium parts of occupation numbers.

$\rho(E)$ is the normalized QP density of states. Throughout simulations it is assumed $\rho(E) = 0$ for $E < \Delta$ and the BCS expression with a finite depairing factor $\rho(E) = Re\left(\frac{E-i\Gamma}{\sqrt{(E-i\Gamma)^2-\Delta^2}}\right)$ for $E \geq \Delta$. Small $\Gamma = 10^{-4}$ is employed, to avoid the divergence of $\rho(\Delta)$ in the numerical procedure and simultaneously to keep the sharpness of the singularity.

$R_n$ - tunnel (normal) resistance of the junction, $R_n = \rho_c s/A$, where $\rho_c = 30\Omega cm$ is the $c-$axis resistivity [7].

$A(E_1, E_2) = 1 - \frac{\Delta^2}{E_1 E_2}$ and $B(E_1, E_2) = 1 + \frac{\Delta^2}{E_1 E_2}$ are the BCS coherence factors.

## II. NONEQUILIBRIUM PHENOMENA IN INTRINSIC JOSEPHSON JUNCTIONS

HTSC intrinsic Josephson junctions form tightly packed stacks of junctions with atomic scale layer thickness $d \sim 4\mathring{A}$ and stacking periodicity $s = 1.5$ nm for Bi-2212. Such stacking leads to strong electromagnetic coupling between IJJs, which causes a number of unusual phenomena, not present in single junctions [8–12].

Discussion of nonequilibrium effects in IJJs has a long history. First, in mid-90's M. Tachiki and L. Bulaevskii with co-workers [13, 14] suggested that charge neutrality could be broken in stacked IJJs, which could add a nonequilibrium term to the ac-Josephson relationship. The nonequilibrium shift of the chemical potential due to charge imbalance on atomically thin layers may be significant, provided that the interlayer spacing is smaller than the Thomas-Fermi screening length [15–17]. This type of disequilibrium was actively studied in connection with Josephson plasma generation [18, 19] and charge imbalance [20] in IJJs. I want to emphasize that the charge disequilibrium in that case is due to collective dynamics of the superconducting condensate in stacked IJJs and is completely different from the nonequilibrium boson generation due to single QP relaxation, considered here. As a matter of fact I do not consider the ac-Josephson effect at all. The phenomena I discuss occur not in the junction but in the electrode. Therefore, one shouldn't confuse those two nonequilibrium effects in IJJs.

Fig. 1 illustrates the type of nonequilibrium effects considered here. It represents the tunneling diagram for two stacked JJs. In this case nonequilibrium QPs are injected in thin superconducting electrodes via tunnel junctions. The QPs decay into the ground state, i.e. recombine into Cooper pairs. The decay typically follows a two-step process [21]: first QP's relax to the edge of the gap, emitting a bremsstrahlung radiation [22]. At the second stage, two QP's from the bottom of the "conduction" band recombine into the Cooper pair, emitting

recombination radiation, as indicated by wavy arrows in Fig. 1.

Importantly, relaxation may occur only via emission of bosons with which QPs have a finite interaction cross-section. Similarly, upon recombination of two QPs into a Cooper pair a bosonic particle, participating in pairing, is emitted. For conventional low-$T_c$ superconductors those are phonons [23]. For HTSC the pairing interaction is not yet confidently known and there are several candidates for bosonic particles that may constitute the spectrum of nonequilibrium emission. Those can be spin waves [24] (magnons in the antiferromagnetic parent state of cuprates), plasmons in case of strong electron-electron correlations [25] and phonons. There is evidence for strong electron-phonon interactions in cuprates [2]. Strong, although unusual isotope effect was reported [26]. Most probably, there is considerable nonequilibrium phonon emission in HTSC as well. In this case relaxation of injected QPs may involve a broad spectrum of both low and high frequency phonons, but recombination should involve high-frequency optical phonons [27] with the wavelength in the interatomic range. Below I will follow a well established electron-phonon formalism of QP relaxation, keeping in mind that it can be adopted to any type of electron-boson interaction.

### A. Factors affecting nonequilibrium population in stacked junctions

In the Introduction I have mentioned that the nonequilibrium QP and boson population in IJJs can be several orders of magnitude larger than in typical LTSC JJs. A very rough estimation could be made assuming that the nonequilibrium QP population $\delta f$ is proportional to the QP injection rate $\partial N_{QP}/\partial t \propto I = JA$, divided by the total DoS in the electrode and multiplied by the effective relaxation time $\tau$. The total DoS is the product of the DoS per unit volume $D_{QP}$ (a material property) and the volume $\mathfrak{V} = Ad$ of the electrode. Therefore, $\delta f \propto J\tau/(dD_{QP})$. It is seen that the following factors affect the magnitude of nonequilibrium population in a single junction:

(i) *The QP injection rate*, which is proportional to the current density through the junction. The superconducting critical current densities in IJJs and Nb-junctions are about the same $J_c \sim 10^2$-$10^3$ (A/cm$^2$) [7]. However, the superconducting energy gap $\Delta \simeq 30$ meV in IJJs [4, 7] is about 20 times more than in Nb. As a result, the current density at the sum-gap voltage $V_g = 2\Delta/e$ is $\sim 10^4$ (A/cm$^2$) in optimally doped Bi-2212 IJJs [4, 7], which is about an order of magnitude larger than $J(V_g)$ in typical Nb junctions and two-three orders of magnitude larger than in typical Al junctions.

(ii) *Atomic thickness of electrodes* $d \simeq 4\mathring{A}$ in IJJs is about two-three orders of magnitude thinner than in LTSC JJs, which proportionally increases nonequilibrium effects.

(iii) The $D_{QP}$ in HTSC materials (which are doped insulators) is several times smaller than in LTSC materials (which are good metals).

(iv) *The relaxation time* in Bi-2212, $\tau \sim$ ps, [27] is much shorter than in Nb, $\tau \sim 10^{-10}$ s, and Al, $\tau \sim \mu$s [28].

Factors (i-iii) tend to increase $\delta f$ in a single IJJ by about four orders of magnitude compared to Nb-junctions and six orders of magnitude compared to Al-junctions. However, this increase is compensates by the shorter $\tau$ so that the magnitude of nonequilibrium effects in a *single* IJJ should be roughly the same as in Al-junctions (which is in general large).

However, *stacking* of IJJs leads to additional enhancement of nonequilibrium population via:

(v) *Cascade amplification of boson population* upon sequential QP tunneling in a stack. It increases $\delta g$ with increasing the number of junctions in the stack [29].

(vi) *Quasiparticle confinement in a stack*: injected QPs rapidly leave the junction area. If QPs depart by more than a mean-free path from the junction they are lost (escape) because they can no longer participate in tunneling or interact with other injected QPs. In typical LTSC materials a ballistic QP flies over the distance of 100 nm in less than 0.1 ps, which is much shorter than the relaxation time $\tau$. Such very fast escape of nonequilibrium QPs is the primary reason for underperformance of superconducting tunnel junction particle detectors [30]. Stacking of IJJs in Bi-2212 mesa structures prevents the escape of nonequilibrium QPs into the bulk pedestal and thus substantially increases the nonequilibrium QP population. It is this effect that I utilize in the presented simulations for the simplest case of a double stack: confinement of injected QPs strongly enhances $\delta f$ at the middle electrode in comparison to the single junction case. Note that such enhancement is not specific to IJJs but was also clearly observed in LTSC stacked JJs [31]. Note also that exactly the same type of confinement of nonequilibrium QPs is used for achieving lasing in semiconducting double heterostructures [32].

Although a rigorous estimation of the enhancement of nonequilibrium effects in stacked IJJs is not yet possible, it is instructive to note that each of the two stacking factors (v,vi) have led to a two orders of magnitude (together - four orders of magnitude) decrease of the threshold current of semiconducting heterostructure lasers [32]. I assume that a similar magnitude of enhancement could be expected for stacked IJJs as well.

## III. THEORY: QUASIPARTICLE AND BOSON KINETIC BALANCE EQUATIONS

The number of excess QPs in the energy interval from $E$ to $E + \delta E$ above the Fermi level is:

$$\delta N(E) = 2\mathfrak{V} D_{QP}(0)\rho(E)\delta f(E)\delta E. \tag{1}$$

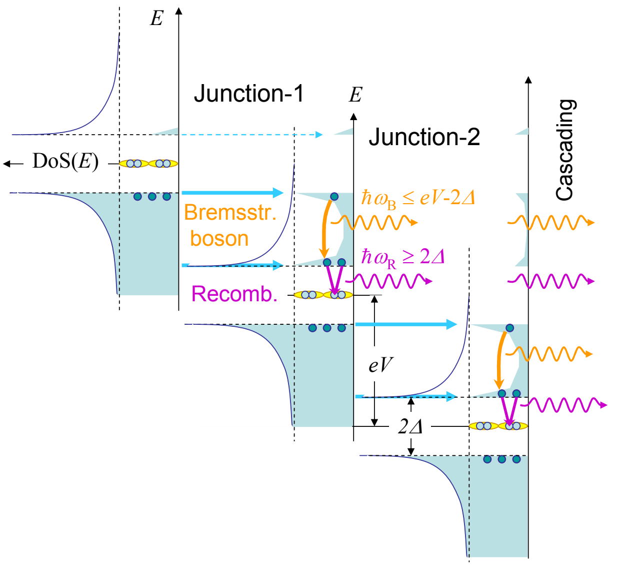


FIG. 1: (Color online) A schematic energy diagram of two stacked SIS junctions biased at voltage $V$ per junction. For $V \geq 2\Delta/e$ tunneling results in nonequilibrium QP population in the empty band. Arrows indicate the most probable relaxation scenario of nonequilibrium QP's. The process is repeated in the second stacked junction, resulting in cascade amplification of radiation, as indicated by wavy arrows.

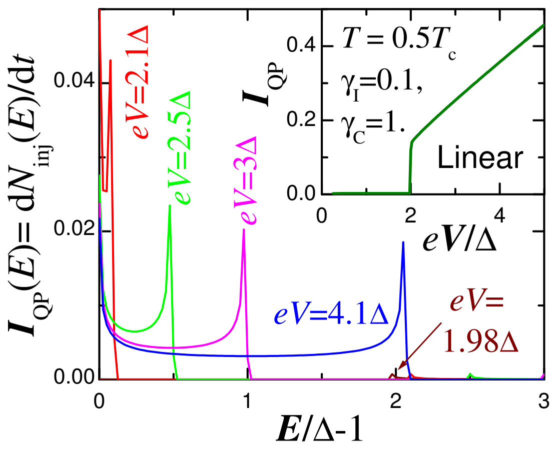


FIG. 2: (Color online). Energy distribution of the equilibrium QP current at different bias voltages (energy is counted from the edge of the gap). Inset shows the corresponding $I-V$ characteristics, in which $I$ is the integral of $I_{QP}(E)$.

Similarly, the number of excess bosons with frequency $\omega$ and energy from $\Omega = \hbar\omega$ to $\Omega + \delta\Omega$:

$$\delta N(\Omega) = \mathfrak{V} N_I D_B(\Omega)\delta g(\Omega)\delta\Omega. \tag{2}$$

Nonequilibrium distributions of QPs and bosons are described by a system of two coupled kinetic equations [33, 34]:

$$\frac{\partial \delta N(\Omega, E)}{\partial t} = \frac{\partial \delta N}{\partial t}_{inj} + \frac{\partial \delta N}{\partial t}_{rel} + \frac{\partial \delta N}{\partial t}_{esc}, \tag{3}$$

which describes dynamic equilibrium between injection, relaxation and escape of the corresponding particles, respectively. I want to emphasize that all terms in those equations are nonlinear. Significance of nonlinearity was emphasized long ago [35].

### A. QP injection and escape rates

Nonequilibrium QPs are injected in electrodes via tunnel junctions. The rate of injection is proportional to the tunneling current:

$$\frac{\partial \delta N(E)}{\partial t}_{inj} = \frac{\Delta}{e^2 R_n}\rho(E)\rho(E-eV)[f(E-eV)-f(E)]\frac{dE}{\Delta}, \tag{4}$$

where $V$ is the bias voltage (per junction). Note that this equation is nonlinear because $\Delta$ depends on $f$ via the nonlinear self-consistency equation, described in sec. F below.

Fig. 2 shows a typical energy distribution of the QP injection rate for different values of the bias voltage for a junction in the equilibrium state at the base temperature $T = 0.5T_c$. The inset show the corresponding QP current-voltage characteristics. Below the sum-gap voltage $V < 2\Delta/e$ only thermally excited (equilibrium) or nonequilibrium QPs contribute to a small current with a sharp maximum at $E = \Delta + eV$, as marked by the dashed horizontal arrow in Fig. 1. It is also marked by the arrow for $eV = 1.98\Delta$ in Fig. 2. For $V > 2\Delta/e$ the injected QP current increases stepwise, as seen from the inset in Fig. 2. The tunnel current has two sharp maxima with equal heights at $E = \Delta$ and $E = eV - 2\Delta$, corresponding to singularities at the gap edge in the two electrodes, as indicated by thick horizontal arrows in Fig. 1.

As for the "escape" process for QPs, it may depend on a specific situation, e.g., in particle detectors it corresponds to diffusion of nonequilibrium QPs sufficiently far away from the tunnel barrier [30]. Here I am mostly interested in a specific case of stacked Josephson junctions with thin electrodes, such as IJJs. In this case nonequilibrium QPs escape predominantly by sequential tunneling into the next junction. Tunnel barriers in stacked junctions effectively block escape of nonequilibrium QPs from the inner electrodes. Therefore leakage (escape) of nonequilibrium QPs is second order (with respect to $\delta f$), compared to the QP injection, and is neglected in the presented simulations (i.e., I assumed $\gamma_Y = 0$).

### B. Boson injection and escape rates

Phonons are traveling in electrodes at the sound velocity $v_s$. Whenever they arrive to the tunnel barrier, they

(with a certain probability) escape from one electrode and are injected in the other. In this case, phonon escape rate is simply proportional to the impingement rate on the barrier. For the frequency window $\Omega - \Omega + dE$ it is given by:

$$\frac{\partial \delta N(\Omega)}{\partial t}_{esc} = -\delta N(\Omega)\frac{v_s}{d} = -\frac{\mathfrak{V}^2 N_I \Delta^3}{2\pi^2\hbar^3 v_s^2 d}\frac{\Omega^2}{\Delta^2}\frac{d\Omega}{\Delta}\delta g(\Omega) \tag{5}$$

Here I used Debye expression for phonon density of states $D_B(\Omega) = (\mathfrak{V}\Omega^2)/(2\pi^2 v_s^3\hbar^3)$.

Specific for stacked atomic-scale IJJs is that phonons, unlike QPs, move freely between the atomic layers and thus are collective for several atomic layers. Therefore, the nonequilibrium distribution of bosons can be amplified in a cascade manner [29] (as indicated in Fig. 1), progressively with the number $N_J$ of sequentially biased stacked junctions, just like photons in the Quantum Cascade Laser [36]. However, in the considered case of only two stacked junctions cascading is not yet significant. Also it was assumed that there is no nonequilibrium boson injection from the outer electrodes ($\gamma_P = 0$). Therefore, the obtained phenomena are generic even for a single junctions.

### C. Relaxation rate of QP's

The formalism of electron-boson relaxation in superconductors has been developed in the famous BCS work:

$$\frac{\partial \delta N(E)}{\partial t}_{rel} = -\frac{4\pi\mathfrak{V}D_{QP}(0)dE}{\hbar}\times$$
$$\int_0^\infty d\Omega\alpha^2(\Omega)D_B(\Omega)\rho(E)\rho(E+\Omega)A(E,E+\Omega)\{f(E)[1-f(E+\Omega)]g(\Omega) - f(E+\Omega)[1-f(E)][\underline{1}+\underbrace{g(\Omega)}]\}$$
$$+\int_0^{E-\Delta} d\Omega\alpha^2(\Omega)D_B(\Omega)\rho(E)\rho(E-\Omega)A(E,E-\Omega)\{f(E)[1-f(E-\Omega)][\underline{1}+\underbrace{g(\Omega)}] - f(E-\Omega)[1-f(E)]g(\Omega)\}$$
$$+\int_{E+\Delta}^\infty d\Omega\alpha^2(\Omega)D_B(\Omega)\rho(E)\rho(\Omega-E)B(E,\Omega-E)\{f(E)f(\Omega-E)[\underline{1}+\underbrace{g(\Omega)}] - [1-f(E)][1-f(\Omega-E)]g(\Omega)\}.$$

Here the first integral describes net scattering upwards with absorption of a boson, the second integral - net relaxation with emission of a boson and the third integral describes pair breaking and recombination. The latter transfer two nonequilibrium QPs into the condensate. Underlined and underbraced terms mark relaxation with spontaneous and stimulated boson emission, respectively. Other terms correspond to absorption of bosons by QPs and pairs. I again emphasize that the QP relaxation is possible only due to non-zero electron-boson spectral function $\alpha$.

### D. Relaxation rate of bosons

Nonequilibrium bosons are produced upon relaxation of nonequilibrium QPs, i.e., there is an exact balance between boson excitation and QP relaxation. Therefore, the boson relaxation rate is opposite to the QP relaxation rate:

$$\frac{\partial \delta N(\Omega)}{\partial t}_{rel} = -\frac{8\pi\mathfrak{V}D_{QP}(0)\alpha^2(\Omega)D_B(\Omega)d\Omega}{\hbar}\times$$
$$\int_\Delta^\infty dE\rho(E)\rho(E+\Omega)A(E,E+\Omega)\{f(E)[1-f(E+\Omega)]g(\Omega) - f(E+\Omega)[1-f(E)][\underline{1}+\underbrace{g(\Omega)}]\}$$
$$+\frac{1}{2}\int_\Delta^\infty dE\rho(E)\rho(\Omega-E)B(E,\Omega-E)\{[1-f(E)][1-f(\Omega-E)]g(\Omega) - f(E)f(\Omega-E)[\underline{1}+\underbrace{g(\Omega)}]\}$$

Here the two terms in each of the two integrals describe absorption or emission of bosons, respectively, caused by relaxation of QPs (the first integral), and by pair break-

ing or recombination (the second integral). The factor 1/2 in front of the second integral reflects the fact that two QPs produce one boson upon recombination into the Cooper pair. Here also underlined and underbraced terms mark spontaneous and stimulated boson emission, respectively.

### E. Expansion of quasiparticle and boson relaxation rates

To simplify the numerical solution, I rewrite the QP and boson relaxation equations in terms of nonequilibrium occupation numbers $\delta f$, $\delta g$:

$$\begin{aligned}\frac{\partial \delta N(E)}{\partial t}_{rel} &= -\frac{4\pi\mathfrak{V}D_{QP}(0)\Delta^4 b}{\hbar}\frac{dE}{\Delta}\times \\ &\int_0^\infty \frac{d\Omega}{\Delta}\frac{\Omega^2}{\Delta^2}\rho(E)\rho(E+\Omega)A(E,E+\Omega)\times \\ &\{\delta f(E)[g(\Omega)+\underline{f(E+\Omega)}]-\delta f(E+\Omega)[\underline{1-F(E)}+\underbrace{g(\Omega)}]+\delta g(\Omega)[F(E)-\underbrace{F(E+\Omega)}]\} \\ &+\int_0^{E-\Delta}\frac{d\Omega}{\Delta}\frac{\Omega^2}{\Delta^2}\rho(E)\rho(E-\Omega)A(E,E-\Omega)\times \\ &\{\delta f(E)[1+\underbrace{g(\Omega)}-\underline{f(E-\Omega)}]-\delta f(E-\Omega)[g(\Omega)+\underline{F(E)}]+\delta g(\Omega)[\underbrace{F(E)}-F(E-\Omega)]\} \\ &+\int_{E+\Delta}^\infty \frac{d\Omega}{\Delta}\frac{\Omega^2}{\Delta^2}\rho(E)\rho(\Omega-E)B(E,\Omega-E)\times \\ &\{\delta f(E)[g(\Omega)+\underline{f(\Omega-E)}]+\delta f(\Omega-E)[g(\Omega)+\underline{F(E)}]+\delta g(\Omega)[F(E)+F(\Omega-E)-1]\}\end{aligned} \tag{6}$$

The corresponding expanded boson relaxation rate is:

$$\begin{aligned}\frac{\partial \delta N(\Omega)}{\partial t}_{rel} &= -\frac{8\pi\mathfrak{V}D_{QP}(0)\Delta^4 b}{\hbar}\frac{d\Omega}{\Delta}\times \\ &\int_\Delta^\infty \frac{dE}{\Delta}\frac{\Omega^2}{\Delta^2}\rho(E)\rho(E+\Omega)A(E,E+\Omega)\times \\ &\{\delta f(E)[\underline{f(E+\Omega)}+g(\Omega)]-\delta f(E+\Omega)[\underline{1-F(E)}+\underbrace{g(\Omega)}]+\delta g(\Omega)[F(E)-\underbrace{F(E+\Omega)}]\} \\ &-\frac{1}{2}\int_\Delta^\infty \frac{dE}{\Delta}\frac{\Omega^2}{\Delta^2}\rho(E)\rho(\Omega-E)B(E,\Omega-E)\times \\ &\{\delta f(E)[g(\Omega)+\underline{f(\Omega-E)}]+f(\Omega-E)[g(\Omega)+\underline{F(E)}]-\delta g(\Omega)[1-F(E)-F(\Omega-E)]\}\end{aligned} \tag{7}$$

Note that both expanded equations are exact. No terms were abandoned, unless they exactly cancel each other. The latter is the case for all terms containing solely the equilibrium terms $F$ and $G$ [33]. Cancelation of those terms is compulsory because equilibrium state can not cause any nonequilibrium effects. Underlined and underbraced terms in Eqs. (6,7) mark spontaneous and stimulated boson emission, respectively. Note that no stimulated emission terms are left in the last recombination/pair breaking integrals, although they were present in the initial unexpanded integrals. It is due to a specific cancelation effect due to which stimulated recombi-

nation is exactly compensated by stimulated pair breaking. However, for single QP relaxation there is no such cancelation and stimulated emission terms are preserved also in the expanded equations.

In previous numerical studies of nonequilibrium phenomena in JJs [33, 34] the QP and phonon relaxation equations were linearized with respect to equilibrium occupation numbers $F(E)$ and $G(\Omega)$, i.e., all $f$ and $g$ terms in Eqs. (6,7) were replaced by $F$ and $G$. Apparently, such linearization is valid only for $\delta f(F) \ll F(E)$, $\delta g(\Omega) \ll G(\Omega)$. However, this is a very strong requirement which is hardly satisfied at low enough $T$ or high enough $E$ and $\Omega$ where $F(E,T), G(\Omega,T) \to 0$. Therefore, linearized equations may fail to describe even weak nonequilibrium state $\delta f(F) \ll 1$, $\delta g(\Omega) \ll 1$.

### F. Self-consistency equation

In the equilibrium state the energy gap $\Delta_0(T)$ is connected to the electron-boson coupling constant $\lambda$ via the BCS self-consistency equation [3]:

$$\frac{1}{\lambda} = \int_{\Delta_0}^{\Omega_D} \frac{tanh\frac{E}{2k_BT}}{\sqrt{E^2-\Delta_0^2}} dE, \tag{8}$$

where $\Omega_D$ is the cut-off (Debye) frequency.

In the nonequilibrium case the self-consistency equation should be written as:

$$\frac{1}{\lambda} = \int_{\Delta}^{\Omega_D} \frac{1-2f(E)}{\sqrt{E^2-\Delta^2}} dE,$$

where both $f(E)$ and $\Delta$ are nonequilibrium. I expand this equation in terms of nonequilibrium part of the distribution function

$$\frac{1}{\lambda} = \int_{\Delta}^{\Omega_D} \frac{tanh\frac{E}{2k_BT}}{\sqrt{E^2-\Delta^2}} dE - 2\int_{\Delta}^{\Omega_D} \frac{\delta f(E)}{\sqrt{E^2-\Delta^2}} dE. \tag{9}$$

Here I used the equality $1-2F(E) = \tanh(E/2k_BT)$.

In order to avoid the problem with the cut-off divergency of those integrals, and to simplify numerical solution of the self-consistency equation, I subtract the equilibrium Eq.(8) from the nonequilibrium Eq.(9). This provides the final implicit nonlinear integral equation, connecting the nonequilibrium gap $\Delta$ with the nonequilibrium distribution function $\delta f(E)$:

$$\int_1^{\infty} \frac{tanh\left(\frac{\varepsilon C(T)}{2}\frac{T}{T_c}\right) - tanh\left(\frac{\varepsilon C(T)}{2}\frac{\Delta}{\Delta_0}\frac{T}{T_c}\right)}{\sqrt{\varepsilon^2-1}} d\varepsilon = -2\int_{\Delta}^{\infty} \frac{\delta f(E)}{\sqrt{E^2-\Delta^2}} dE. \tag{10}$$

All the integrals in the above equation are well behaving and rapidly converging. Therefore, cut-off frequency is no longer significant and is expanded to infinity. All material parameters are now comfortably encoded in the equilibrium BCS value $C(T) = \Delta_0(T)/k_BT_c$.

## IV. NUMERICAL PROCEDURE

Here is a sketch of the numerical procedure used for solution of the system of two coupled integral equations (3) together with the self-consistency Eq.(10). I follow the discretization procedure introduced in Refs. [33, 34] for solution of linearized equations. I also adopt the nomenclature of Ref. [33].

First, integrals in the relaxation rates Eqs.(6,7) and the self-consistency Eq. (10) were discretized into sums for QP and boson levels with separation $dE = \Delta/K_\Delta$ and the total number of levels $K$ for quasiparticles and $K+2K_\Delta$ for bosons:

$$E_i = \Delta + (i-1)dE,\ (i = 1,2,\cdots K)$$
$$\Omega_j = (j-1)dE,\ (j = 1,2,\cdots K+2K_\Delta).$$

Nonequilibrium parts of QP and boson distribution functions were implemented in an array $x_i$ of length $2K+2K_\Delta$:

$x_i(1 \le i \le K) = \delta f(E_i)$,

$x_{i+K}(1 \le i \le K+2K_\Delta) = \delta g(\Omega_i)$.

Thus integral kinetic equations for QPs and bosons Eq.(3) are substituted by two coupled systems of *nonlinear* equations:

$$R_{ij}\ x_j + \gamma_Y \rho(E_i) x_i = \gamma_I Y_i, \tag{11}$$

$$R_{i+K,j}\ x_j + \gamma_U d_B(\Omega_j) x_{i+K} = \gamma_P Y_{i+K}. \tag{12}$$

Here $(1 \le i \le K)$ and $(1 \le j \le 2K+2K_\Delta)$

In Eqs.(11, 12) the matrix $R_{ij}$ represents the discreetized QP $(1 \le i \le K)$ and boson $(K+1 \le j \le 2K)$ relaxation integrals Eqs.(6, 7), respectively:

$$R_{i,i}=\sum_{j=i}^{K}A_{ij}(G_{l1}+F_j+x_{l1'}+x_j)+\sum_{j=1}^{i}A_{ij}(G_{l2}+1-F_j+x_{l2'}-x_j)+\sum_{j=1}^{K-i+1}2B_{ij}(G'_{l3}+F_j+x_{l3'}+x_j),$$

$$R_{i,j}=\sum_{j=i}^{K}A_{ij}(F_i-1-G_{l1}-x_{l1'})\}-\sum_{1}^{i}A_{ij}(F_i+G_{l2}+x_{l2'})+\sum_{1}^{K-i+1}2B_{ij}(F_i+G'_{l3}+x_{l3'}),$$

$$R_{i,l1'}=\sum_{j=i}^{K}A_{ij}(F_i-F_j),\quad R_{i,l2'}=\sum_{j=1}^{i}A_{ij}(F_i-F_j),\quad R_{i,l3'}=-\sum_{j=1}^{K-i+1}2B_{ij}(1-F_i-F_j),$$

where $i=1,2,\cdots K$, $l1=j-i+1$, $l1'=l1+K$, $l2=i-j+1$, $l2'=l2+K$, $l3=i+j-1$, $l3'=l3+K+2K_d$

$$R_{l',l'}=\sum_{i=1}^{K-l+1}A_{ij1}(F_i-F_{j1}),\quad R_{l',i}=\sum_{i=1}^{K-l+1}A_{ij1}(G_l+F_{j1}+x_{l'}+x_{j1}),\quad R_{l',j1}=\sum_{i=1}^{K-l+1}A_{ij1}(F_i-1-G_l-x_{l'})\},$$

$$R_{l4,l4}=\sum_{i=1}^{l}B_{ij2}(1-F_i-F_{j2}),\quad R_{l4,i}=-\sum_{i=1}^{l}B_{ij2}(G'_l+F_{j2}+x_{l4}+x_{j2}),\quad R_{l4,j2}=-\sum_{i=1}^{l}B_{ij2}(F_i+G'_l+x_{l4}),\tag{13}$$

where $l=1,2,\cdots K$, $l'=l+K$, $l4=l+K+2K_\Delta$, $j1=i+l-1$, $j2=l-i+1$, and

$$A_{ij}=\frac{dE}{\Delta}\frac{(E_i-E_j)^2}{\Delta^2}\rho(E_i)\rho(E_j)\left(1-\frac{\Delta^2}{E_iE_j}\right)$$
$$B_{ij}=\frac{dE}{2\Delta}\frac{(E_i+E_j)^2}{\Delta^2}\rho(E_i)\rho(E_j)\left(1+\frac{\Delta^2}{E_iE_j}\right)\tag{14}$$

Second terms in Eqs.(11, 12) represent the escape rates of QPs and bosons, respectively. To avoid energy dependence of escape coefficients $\gamma_Y$ and $\gamma_U$, they are scaled by the corresponding normalized density of states $\rho(E_i)$ and $d_B(\Omega_j)=(\Omega_j/\Delta)^2$, respectively.

Right-hand sides of Eqs. (11,12) represent the injection rates of QPs Eq.(4) and bosons, respectively.

Coefficients in Eq.(11,12) are:

$$\gamma_I=\frac{\hbar}{4\pi\mathfrak{V}R_ne^2D_{QP}(0)b\Delta^2dE},\tag{15}$$

which controls the rate of injection of QPs via tunneling, relative to the relaxation rate.

$\gamma_Y$ controls the relative rate of escape of QPs via sequential tunneling into the next junction, see Fig. 1, and as explained in sec. II A, was set to zero in simulations.

$$\gamma_U=\frac{3N_I\hbar v_s}{8\pi D_{QP}(0)b\Delta\Omega_D^3 s},\tag{16}$$

controls the rate of escape of ballistic bosons though the junction.

$\gamma_P$ controls the rate of injection of ballistic bosons though the junction, and, as explained in sec. II B, was set to zero in simulations.

In the simulations presented here I used the mesh size $\delta E=\Delta/40$, $K_\Delta=40$, and the maximum energy interval (band width) of $E=12\Delta$ above the Fermi level for quasiparticles and $\Omega=13\Delta$ for bosons. Such large energy intervals were necessary for the analysis of nonequilibrium states at high voltages up to $V=5\Delta/e$.

The obtained system of nonlinear equations for QPs and bosons, together with the self-consistency equation was solved by an iterative procedure in which the obtained $\delta f(E)$ and $\delta g(\Omega)$ at each stage was added to nonequilibrium distribution terms $f$ and $g$ in the matrix $R_{ij}$. After each iteration, the accuracy of solution was checked explicitly by back substitution into the kinetic equations. The absence of spurious effects in the numerical procedure was checked by changing the mesh size, $K_\Delta$, and the energy interval $K$.

## V. ESTIMATION OF NUMERICAL COEFFICIENTS

Using definitions and typical Bi-2212 parameters specified in Sec.I, and the mesh size $dE=\Delta/40$ used in numerical simulations, we can make a rough estimation of coefficients in the numerical scheme for the case of

Bi-2212 IJJs.

The QP injection coefficient Eq.(15):

$$\gamma_I \simeq 0.04. \tag{17}$$

From Eq.(15) it follows that $\gamma_I$ increases rapidly $\propto \Delta^{-3}$ with decreasing the gap and can easily reach unity at elevated $T$.

The QP escape and boson injection were neglected: $\gamma_Y = \gamma_P = 0$.

The boson (phonon) escape coefficient Eq.(16):

$$\gamma_U \simeq 0.2. \tag{18}$$

Since the escape rate Eq.(5) is calculated assuming that all phonons are flying towards the junction, the estimated value of $\gamma_U$ can be strongly overestimated, if the majority of phonons have the in-plane velocity. On the other hand, it can also be underestimated if the emitted are not slow phonons but electronic excitations with about two orders of magnitude larger velocities (of the order of the Fermi velocity). In the presented simulations I used $\gamma_U \simeq 0.1$, which corresponds to 50% probability of boson escape upon impingement on the tunnel barrier. It was also assumed that $\gamma_U$ decreased stepwise at high frequencies $\Omega > 2\Delta$, to mimic slowing down of high frequency acoustic and optical phonons.

Due to crudeness of approximations made above, those estimations are accurate to within an order of magnitude, at most. Thus, I do not pretend on making a numerical fit for Bi-2212. Rather, my goal is to study basic nonlinear nonequilibrium effects in Josephson junctions. Therefore, during simulations I have varied numerical coefficients in a wide range, independently from each other.

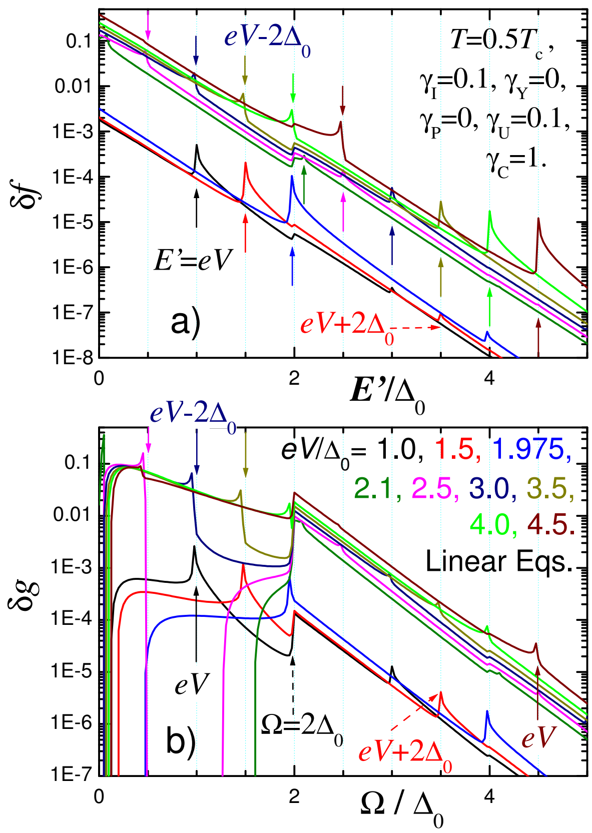


FIG. 3: (Color online). Solution of linearized kinetic equations for junctions with the same parameters as in Fig. 2 at different bias voltages. Panels a) and b) show energy distributions of nonequilibrium QP (energy counted from the edge of the gap) and boson populations, respectively.

## VI. LINEAR APPROXIMATION

To cope with previous works [33, 34], below I show solutions of the linearized versions of kinetic equations. They represent the first iteration in the numerical procedure, which starts from $f = F$ and $g = G$ in Eqs. (6,7). To keep the problem fully linear, I also skip at this stage the self-consistency equation. This simplification does not cause any qualitative difference in the linear solution.

Fig. 3 represents the linear solution at the base temperature $T/T_c = 0.5$, for QP injection coefficient $\gamma_I = 0.1$, no QP escape $\gamma_Y = 0$, boson escape coefficient $\gamma_U = 0.1$ and no boson injection $\gamma_P = 0$ (the boson current is absent in the linear approximation because it assumes $\delta g = 0$, thus the value $\gamma_P$ does not play any role here).

Fig. 3 a) shows the nonequilibrium QP distribution as a function of energy, counted from the edge of the gap, $E' = E - \Delta$, for several bias voltages. The corresponding QP injection rates are shown in Fig. 2. I refer to the tunneled QPs as the "primary" nonequilibrium QPs. At $eV < 2\Delta$ the QP current is due to solely thermally excited QPs in the QP "conductance" band, as indicated by the dashed horizontal arrow on the diagram for junction-1 in Fig. 1. This results in appearance of a small, almost bias independent primary QP peak in $\delta f$ at $E' = eV$, marked by upward arrows in Fig. 3 a). At $eV > 2\Delta$, the QP current increases stepwise, as seen from the inset in Fig. 2, and the injected QP rate acquires two equally strong peaks at $E' = 0$ and $E' = eV - 2\Delta$, as shown in Fig. 2. This leads to a dramatic increase of $\delta f$ and appearance of the strong primary QP peak in $\delta f$ at $E' = eV - 2\Delta$, marked by downward arrows in Fig. 3 a).

However, the position of the peak is the only similarity between the injection rate of primary QPs and the final distribution of nonequilibrium QPs. It is seen that $\delta f(E)$ is substantially different from $dN_{inj}(E)/dt$: $\delta f(E)$ has a maximum at $E' = 0$, i.e., at the bottom of the "conductance band", and decays roughly exponentially with $E'$. Taking into account that the total number of nonequilibrium QPs scales with the density of states $\rho(E)$, which has a singularity at $E' = 0$, it becomes clear that the vast majority of nonequilibrium QPs are residing just at the edge of the gap. This happens because in the considered case without QP escape, recombination is the only sink

channel for QPs. It forms a bottleneck for removal of nonequilibrium QPs and leads to their accumulation at the bottom of the QP conductance band.

Fig. 3 b) shows the nonequilibrium boson distribution as a function of energy for the same bias voltages as in a). We can clearly identify primary and secondary features in the nonequilibrium boson spectra:

1) Relaxation of primary QPs leads to appearance of the primary bosonic bremsstrahlung band with $0 \leqslant \Omega \leqslant eV - 2\Delta$ at $eV > 2\Delta$. The bosonic spectrum has a maximum at the edge of the bremsstrahlung band $\Omega = eV - 2\Delta$ for $eV > 2\Delta$, (indicated by solid downward arrows in Fig. 3 b), which corresponds to direct fall of primary QPs with maximum injection rate at $E' = eV - 2\Delta$, see Fig. 2, to the bottom of the conduction band. A small peak in $\delta g$ at $\Omega = eV$ (indicated by solid upward arrows in Fig. 3 b) is due to a similar direct fall of tunneled thermally excited QPs.

2) Recombination of nonequilibrium QPs into Cooper pairs leads to appearance of a continuous recombination bosonic band with $\Omega \geqslant 2\Delta$. The recombination spectrum has a clear maximum at the edge of the band $\Omega = 2\Delta$, which corresponds to recombination of two QPs from the edge of the gap (bottom of conductance band).

Appearance of the maxima at the edges of bosonic bremsstrahlung and recombination bands, $\Omega = eV - 2\Delta$ and $\Omega = 2\Delta$, indicates the most usual QP relaxation steps: first, QPs fall directly to bottom of the conduction band, and then recombine therefrom into Cooper pairs. Predominance of those processes are due to the BCS singularity in the QP DoS at the edge of the gap. It is better seen from the total number of nonequilibrium bosons (scaled by the bosonic Debye DoS $D_B \propto \Omega^2$) which has sharp absolute maxima at the corresponding frequencies, see Fig. 2 (a) in the main manuscript.

From Fig. 3 we can also see appearance of the following secondary nonequilibrium particles: reabsorption of recombination bosons by QPs leads to appearance of secondary QPs with maximum in $\delta f$ at $E' = 2\Delta$, and a smaller peak at $E' = eV + 2\Delta$, marked by the dashed arrow in Fig. 3 a). Relaxation of the latter to the edge of the gap leads to emission of secondary bosons with a maxima in $\delta g$ at $\Omega = eV + 2\Delta$, marked by the dashed arrow in Fig. 3 b).

There are other weaker processes, which do not lead to sharp features, but nevertheless visible in the spectra. For example, from Fig. 3 b) it is seen that at $eV$ slightly above $2\Delta$, e.g., for $eV = 2.1\Delta$ and $2.5\Delta$, the two bosonic bands are perfectly separated. This reflects the lack of QPs injection at $E' > eV - 2\Delta$, see Fig. 2. As a matter of fact $\delta g$ acquires a small negative value between the bands, i.e. there is a net absorption of thermal-equilibrium bosons by nonequilibrium QPs in this frequency range. However, at higher bias, see e.g. the curve for $eV = 3\Delta$ in Fig. 3 b), the bosonic spectrum at $eV - 2\Delta < \Omega < 2\Delta$ is not empty, which is due to a secondary, two stage, process in which the injected QP firsts gains energy by absorbing either an equilibrium or a primary nonequilibrium boson and then relaxes by emission of the secondary boson with energy $\Omega > eV - 2\Delta$. Other secondary processes lead to small peaks in $\delta g$ at $\Omega = 4\Delta$ and $eV + 2\Delta$.

All described peculiarities occur also in the nonlinear solution, although with different amplitudes.

---


[1] V.Z.Kresin and S.A.Wolf, *Phys. Rev. B* **41**, 4278 (1990); P. Mandal, A. Poddar, B. Ghosh, and P. Choudhury, *Phys. Rev. B* **43**, 13102 (1991).

[2] R.S. Gonnelli, G.A. Ummarino, and V.A. Stepanov, *Physica C* **275**, 162 (1997); E.G.Maksimov, O.V.Dolgov, and M.L.Kulic, *Phys. Rev. B*, **72**, 212505 (2005); M.L.Kulic, and O.V.Dolgov, *ibid.* **76**, 132511 (2007); C. Falter, *Phys. Stat. Sol.* **242**, 78 (2005).

[3] J.P. Carbotte, *Rev. Mod. Phys.* **62**, 1027 (1990).

[4] V.M. Krasnov, A. Yurgens, D. Winkler, P. Delsing and T. Claeson, *Phys. Rev. Lett.* **84**, 5860 (2000); V.M. Krasnov, A.E. Kovalev, A. Yurgens and D. Winkler *ibid.* **86**, 2657 (2001).

[5] J. Wu, Y.N. Wang, P.S. Guo, H.M. Shen, Y.F. Yan, and Z.X. Zhao, *Phys. Rev. B* **47**, 2806 (1993).

[6] A. Damascelli A, Z. Hussain, and Z.X. Shen, *Rev. Mod. Phys.* **75**, 473 (2003)

[7] V.M. Krasnov, *Phys. Rev. B* **65**, 140504(R) (2002); *ibid.* **79**, 214510 (2009).

[8] S. Sakai, P.Bodin and N.F. Pedersen, *J. Appl. Phys.* **73**, 2411 (1993).

[9] R. Kleiner, *Phys. Rev. B* **50**, 6919 (1994).

[10] V.M. Krasnov, V.A.Oboznov, V.V. Ryazanov, N. Mros, A. Yurgens, and D. Winkler, *Phys. Rev. B* **61**, 766 (2000).

[11] M. Machida, T. Koyama, A. Tanaka, and M. Tachiki, *Physica C* **330**, 85 (2000); M. Machida, *Phys. Rev. Lett.* **96**, 097002 (2006).

[12] A.E. Koshelev, *Phys. Rev. B* **66**, 224514 (2002).

[13] M. Tachiki, T. Koyama and S.Takahashi, *Phys. Rev. B* **50**, 7065 (1994).

[14] L.N. Bulaevskii, M. Zamora, D. Baeriswyl, H. Beck, and J.R. Clem *Phys. Rev. B* **50**, 12831 (1994); L.N. Bulaevskii, M.P. Maley and M. Tachiki *Phys. Rev. Lett.* **74**, 801 (1995).

[15] T. Koyama and M. Tachiki, *Phys. Rev. B* **54**, 16183 (1996); M.Machida, T. Koyama and M. Tachiki *Phys. Rev. Lett.* **83**, 4618 (1999).

[16] S.N. Artemenko and A.G. Kobelkov *Phys. Rev. Lett.* **78**, 3551 (1997).

[17] D.A. Ryndyk *Phys. Rev. Lett.* **80**, 3376 (1998); J.Keller and D.A.Ryndyk, *Phys. Rev. B* **71**, 054507 (2005).

[18] Y. Matsuda, M.B. Gaifullin, K.I. Kumagai, M. Kosugi and K. Hirata *Phys. Rev. Lett.* **78**, 1972 (1997); more references on Josephson plasma resonance can be found in a dedicated special issue *Physica C* **364** (2001).

[19] Yu.M. Shukrinov, and F.Mahfouzi *Phys. Rev. Lett.* **98**, 157001 (2007).

[20] S. Rother, Y.Koval, P. Müller, R.Kleiner, D.A. Ryndyk,

J. Keller, and C.Helm *Phys. Rev. B* **67**, 024510 (2003).
[21] W.E. Bron, *Rep. Prog. Phys.* **43**, 20 (1980).
[22] H. Kinder, *Phys. Rev. Lett.* **28**, 1564 (1972).
[23] W. Eisenmenger and A.H. Dayem, *Phys. Rev. Lett.* **18**, 125 (1967).
[24] Ar.Abanov, A.V.Chubukov, and M.R.Norman, *Phys. Rev. B* **78**, 220507(R) (2008).
[25] A.Bill, H.Morawitz and V.Z.Kresin, *Phys. Rev. B* **68**, 144519 (2003); A.N.Pasupathy, et al., *Science* **320**, 196 (2008).
[26] J.Lee, et al., *Nature* **442**, 546 (2006), H.Iwasawa, et al., *Phys. Rev. Lett.* **101**, 157005 (2005).
[27] C.Giannetti, G.Coslovich, F.Cilento, G.Ferrini, H. Eisaki, N. Kaneko, M. Greven, and F. Parmigiani, *Phys. Rev. B* **79**, 224502 (2009); R.P. Saichu, I. Mahns, A. Goos, S. Binder, P. May, S.G. Singer, B. Schulz, A. Rusydi, J. Unterhinninghofen, D. Manske, P. Guptasarma, M.S. Williamsen, and M. Rübhausen, *Phys. Rev. Lett.* **102**, 177004 (2009); L. Perfetti, P.A. Loukakos, M. Lisowski, U. Bovensiepen, H. Eisaki, and M. Wolf, *Phys. Rev. Lett.* **99**, 197001 (2007).
[28] S.B. Kaplan *et al.*, *Phys. Rev. B* **14**, 4854 (1976).
[29] V.M.Krasnov, *Phys. Rev. Lett.* **97**, 257003 (2006).
[30] A.A.Golubov, et al., *Phys. Rev. B* **49**, 12953 (1994).
[31] M.G. Blamire, E.C.G. Kirk, J.E. Evetts, and T.M. Klapwijk, *Phys. Rev. Lett.* **66**, 220 (1991); I.P. Nevirkovets, S.E. Shafranjuk, O. Chernyashevskyy and J.B. Ketterson, *Phys. Rev. B* **76**, 184520 (2007).
[32] Z.I. Alferov, *Rev. Mod. Phys.* **73**, 767 (2001).
[33] A.H. Dayem and J.J. Wiegand, *Phys. Rev. B* **5**, 4390 (1972).
[34] J.J. Chang and D.J. Scalapino, *Phys. Rev. B.* **15**, 2651 (1977); *ibid.* 21, 2045 (1980).
[35] A.Rothwarf and B.N. Taylor, *Phys. Rev. Lett.* **19**, 27 (1967).
[36] J. Faist, et al., *Science* **264**, 553 (1994).
